# Supplementary material for: Electron spin secluded inside a bottom-up assembled standing metal-molecule nanostructure
Source: arXiv:2301.11762 source file (2023-01-27)
Supplement: Supplementary file 1 [file supplement.pdf]

# Supplementary Material to
# Electron spin secluded inside a bottom-up assembled standing metal-molecule nanostructure

Taner Esat,[1,2,*] Markus Ternes,[1,2,3] Ruslan Temirov,[1,2,4] and F. Stefan Tautz[1,2,5]

[1] *Peter Grünberg Institute (PGI-3), Forschungszentrum Jülich, 52425 Jülich, Germany*
[2] *Jülich Aachen Research Alliance (JARA), Fundamentals of Future Information Technology, 52425 Jülich, Germany*
[3] *Institute of Physics II B, RWTH Aachen University, 52074 Aachen, Germany*
[4] *Institute of Physics II, University of Cologne, 50937 Cologne, Germany*
[5] *Experimental Physics IV A, RWTH Aachen University, 52074 Aachen, Germany*

## DYNAMICAL COULOMB BLOCKADE AT MK TEMPERATURES

The dynamical Coulomb blockade (DCB) can be observed in the scanning tunneling microscope (STM) at very low temperatures. It results from the inelastic interaction of the tunneling electrons with the electromagnetic environment in which the junction is embedded [1]. In the differential conductance ($dI/dV$) spectra, it manifests itself as a dip at zero bias [2, 3]. In our Jülich Quantum Microscope [4] we typically observe the DCB at temperatures $\lesssim 250\,\mathrm{mK}$. As can be seen in Fig. S1, the DCB dip is clearly evident in the $dI/dV$ spectra on the standing metal-molecule nanostructure as well as on the Ag(111) surface. We have removed the DCB dip from all $dI/dV$ spectra on the standing nanostructure. For this purpose, we scaled the $dI/dV$ spectrum that was measured on the Ag(111) surface to the background conductance of the respective $dI/dV$ spectrum on the standing nanostructure. Afterwards, we divided the $dI/dV$ spectrum on the standing nanostructure by the spectrum taken on the Ag surface. Finally, we rescaled the obtained $dI/dV$ spectrum back to the original background conductance on the standing nanostructure.

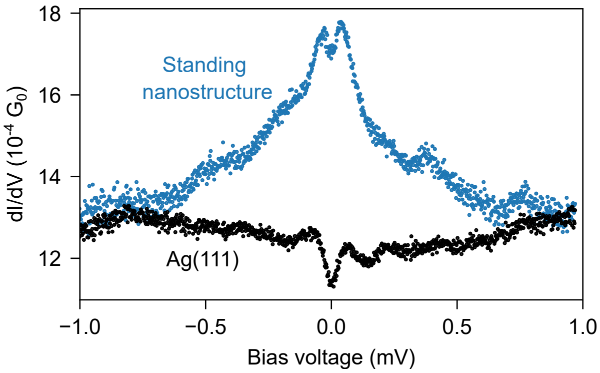


FIG. S1. $dI/dV$ conductance spectra on a standing metal-molecule nanostructure (blue) and on the Ag(111) surface (black) measured at $T \simeq 50\,\mathrm{mK}$ ($V_{\mathrm{mod}} = 20\,\mu\mathrm{V}$). The tip was stabilized at $I_T = 100\,\mathrm{pA}$ and $V = -1\,\mathrm{mV}$. The spectrum on the standing nanostructure corresponds to the spectrum in Fig. 2a at $B = 80\,\mathrm{mT}$.

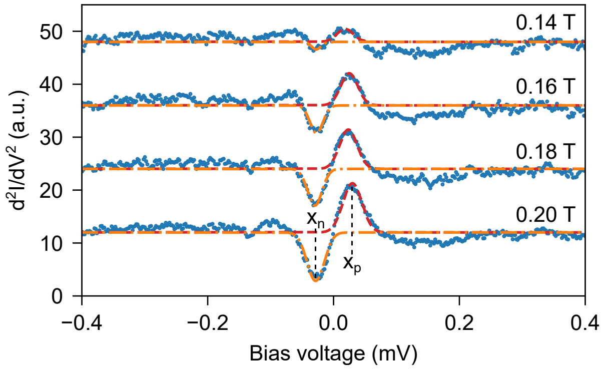


FIG. S2. $d^2I/dV^2$ spectra (blue) on a standing metal-molecule nanostructure after applying a second-order Savitzky-Golay filter to the $dI/dV$ spectra and calculating the numerical derivative. These data correspond to the $dI/dV$ spectra in Fig. 2a. The red (orange) dashed lines illustrate the Gaussian fits to the peaks at positive (negative) bias voltage. The spectra are vertically displaced for clarity.

## DETERMINATION OF THE ZEEMAN ENERGY

In order to extract the precise energy of the Zeeman splitting $\Delta$, we first smoothed the $dI/dV$ spectra measured on the standing metal-molecule nanostructure with a second-order Savitzky-Golay filter, which performs a polynomial fit on a sliding window. To avoid filtering out meaningful signals from the $dI/dV$ spectra, we use a sliding window of only $50\mu$V width. Afterwards, we calculated the numerical derivative of the $dI/dV$ spectra, i.e., $d^2I/dV^2$. In the $d^2I/dV^2$ spectra, the peaks correspond to the steepest slope of the steps arising from inelastic spin-flip excitations in the $dI/dV$ spectra. To determine the exact position $x_p$ ($x_n$) of the peaks, we fitted them at positive (negative) bias voltage with a Guassian. Fig. S2 shows the resulting fits for the data shown in Fig. 2a as an example. Finally, we calculated the Zeeman energy as $\Delta = (|x_n| + |x_p|)/2$.

* Corresponding author: t.esat@fz-juelich.de

[1] H. Grabert and M. H. Devoret, *Single charge tunneling: Coulomb blockade phenomena in nanostructures*, Vol. 294 (Springer Science & Business Media, 2013).

[2] C. R. Ast, B. Jäck, J. Senkpiel, M. Eltschka, M. Etzkorn, J. Ankerhold, and K. Kern, Sensing the quantum limit in scanning tunnelling spectroscopy, Nature Communications **7**, 13009 (2016).

[3] J. Senkpiel, J. C. Klöckner, M. Etzkorn, S. Dambach, B. Kubala, W. Belzig, A. L. Yeyati, J. C. Cuevas, F. Pauly, J. Ankerhold, C. R. Ast, and K. Kern, Dynamical Coulomb blockade as a local probe for quantum transport, Phys. Rev. Lett. **124**, 156803 (2020).

[4] T. Esat, P. Borgens, X. Yang, P. Coenen, V. Cherepanov, A. Raccanelli, F. S. Tautz, and R. Temirov, A millikelvin scanning tunneling microscope in ultra-high vacuum with adiabatic demagnetization refrigeration, Review of Scientific Instruments **92**, 063701 (2021).
